# Supplementary material for: MIMDE: Exploring the Use of Synthetic vs Human Data for Evaluating Multi-Insight Multi-Document Extraction Tasks
Source: arXiv:2411.19689 source file (2024-11-29)
Supplement: Supplementary file 1 [file A-appendix.tex]

\section{Appendix}
\label{sec:appendix}
